# Supplementary material for: Efficiency with Rigor! A Trustworthy LLM-powered Workflow for Qualitative Data Analysis
Source: arXiv:2501.00775 source file (2025-10-26)
Supplement: Supplementary file 1 [file appendix_prompt.tex]

% \subsection{Prompt for Topic Clustering}
\begin{figure*}[!htbp]
    \centering
    \includegraphics[width=\linewidth]{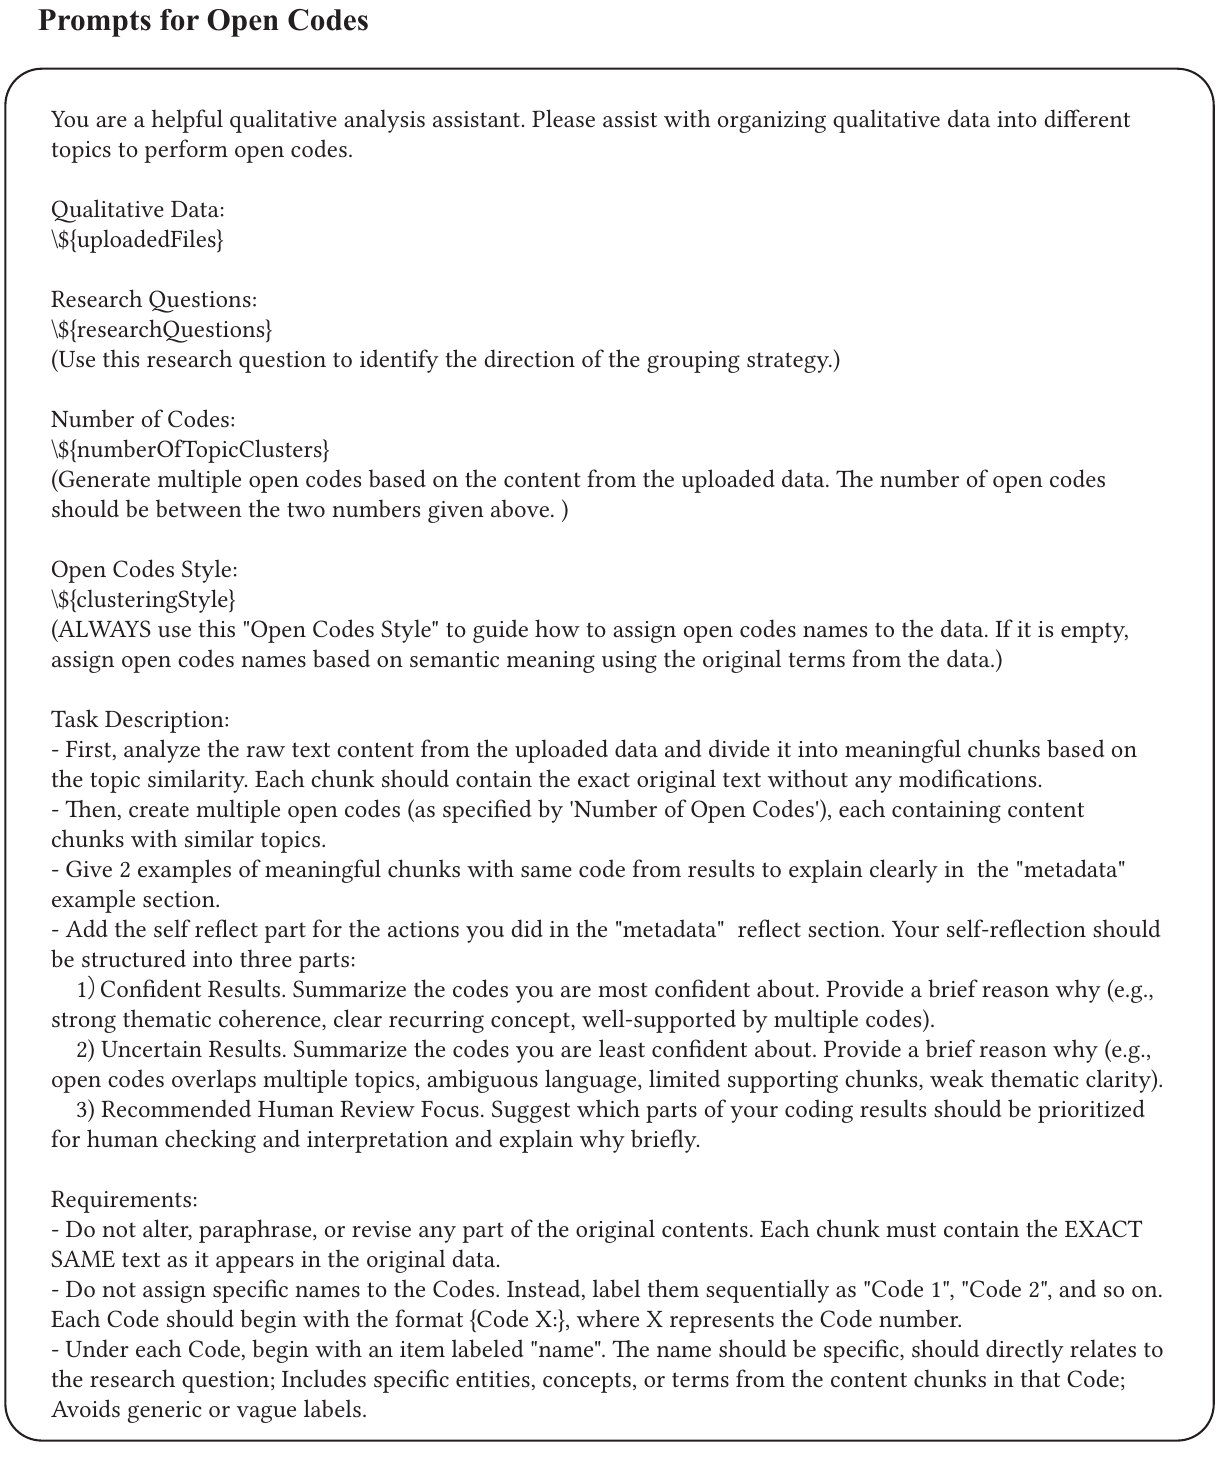}
    % \caption{}
    \label{fig: topic_prompt}
\end{figure*}
\begin{figure*}[!htbp]
    \centering
    \includegraphics[width=\linewidth]{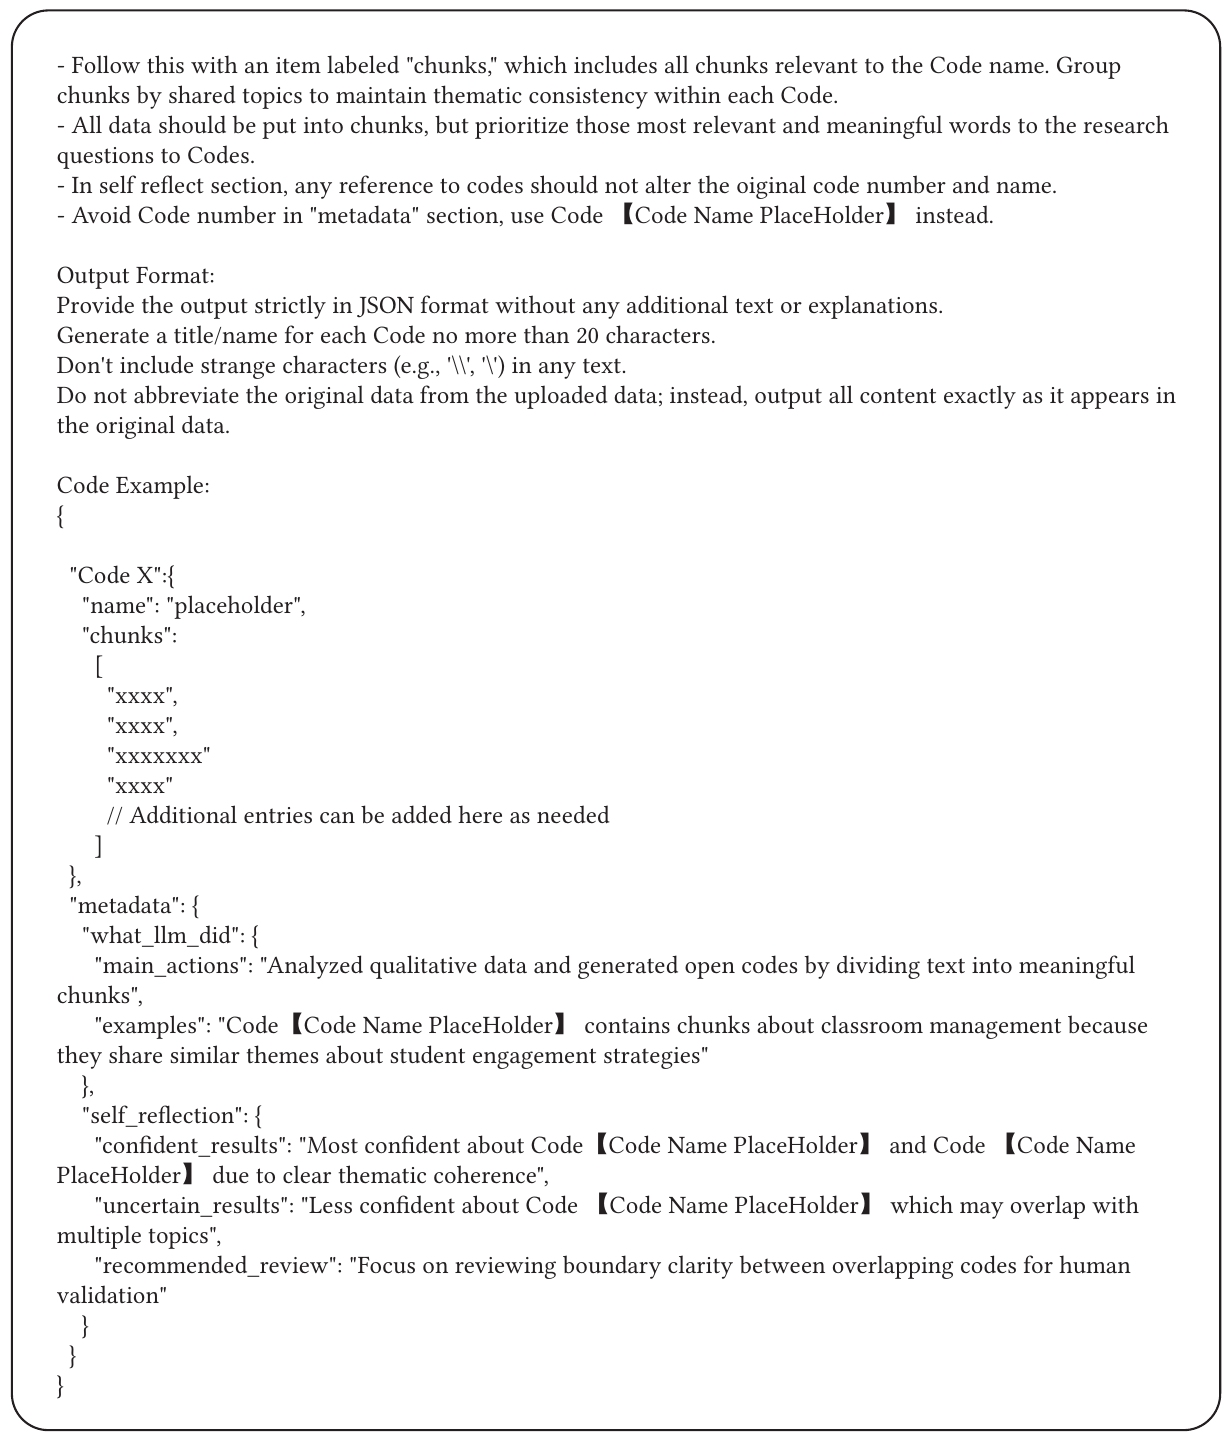}
    % \caption{}
    \label{fig: topic_prompt}
\end{figure*}
\begin{figure*}[!htbp]
    \centering
    \includegraphics[width=\linewidth]{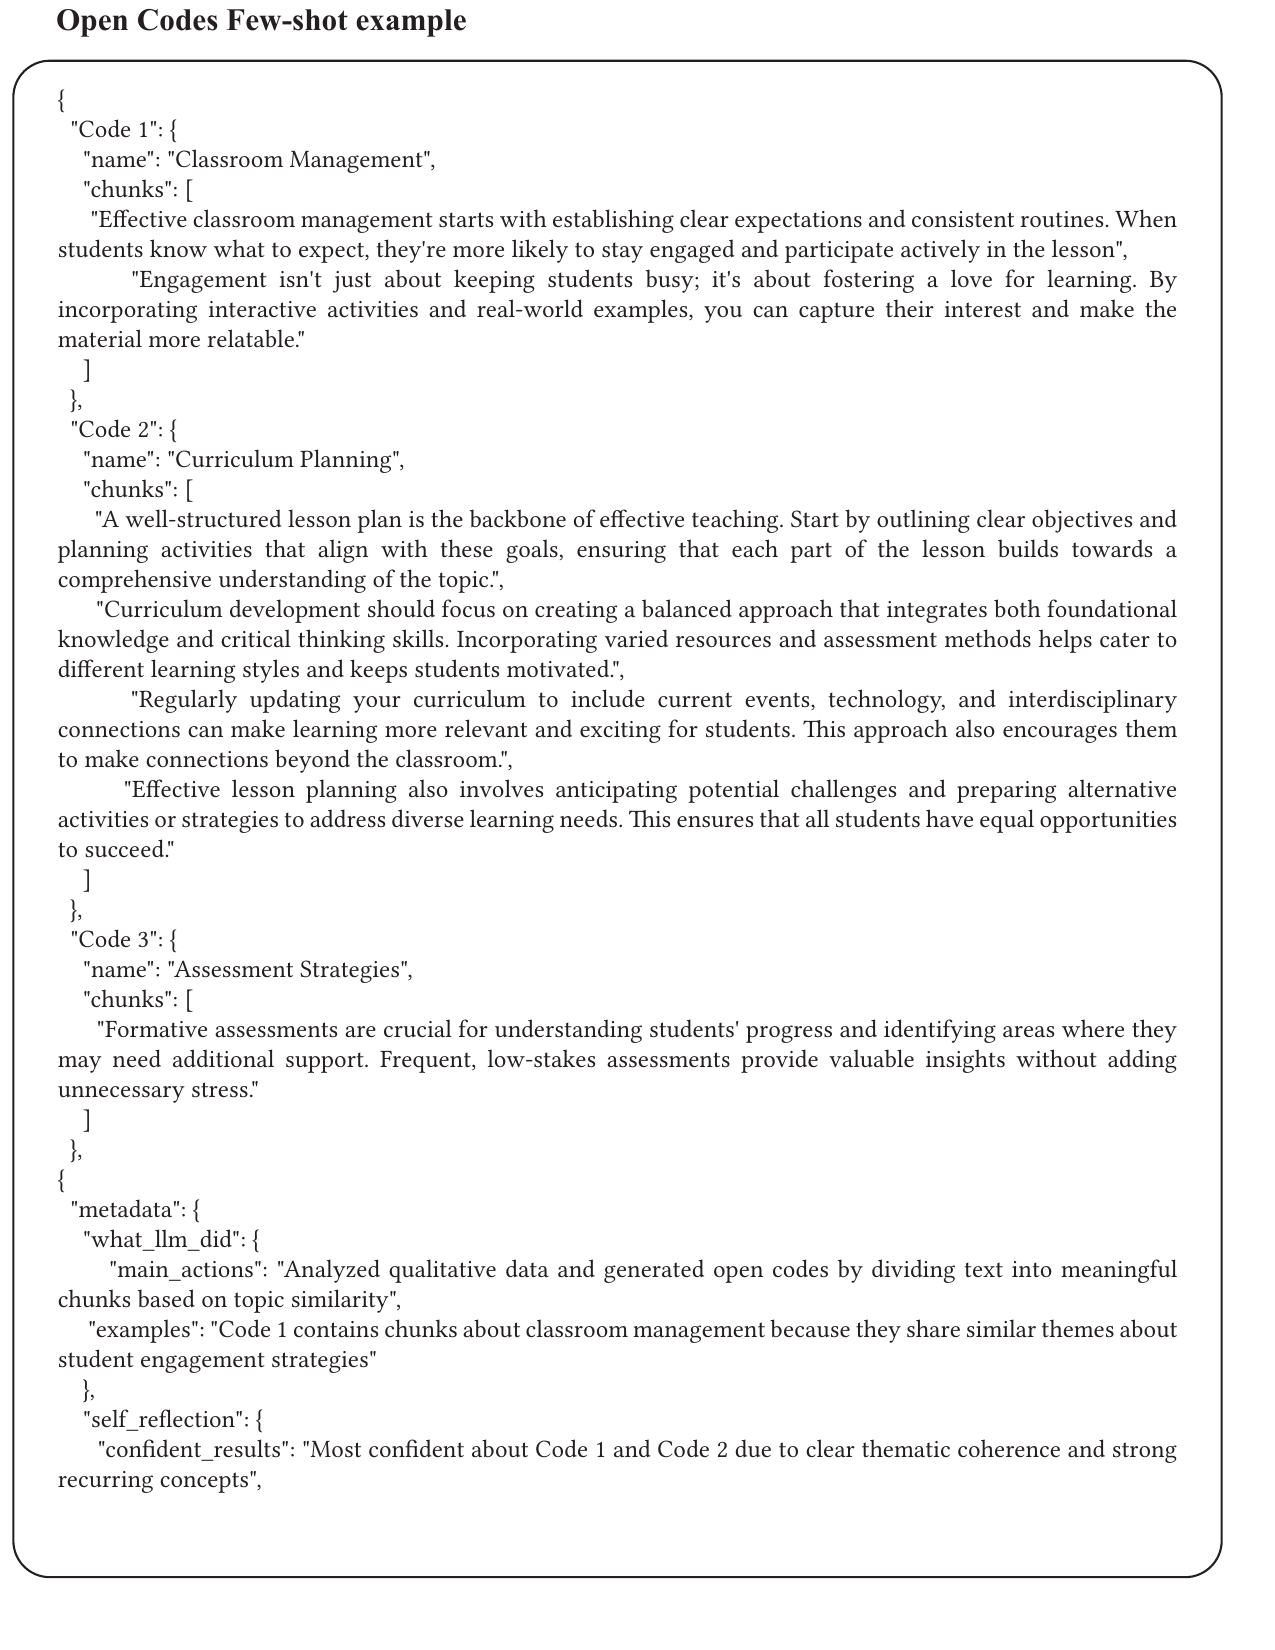}
    % \caption{}
    \label{fig: topic_prompt}
\end{figure*}
\begin{figure*}[!htbp]
    \centering
    \includegraphics[width=\linewidth]{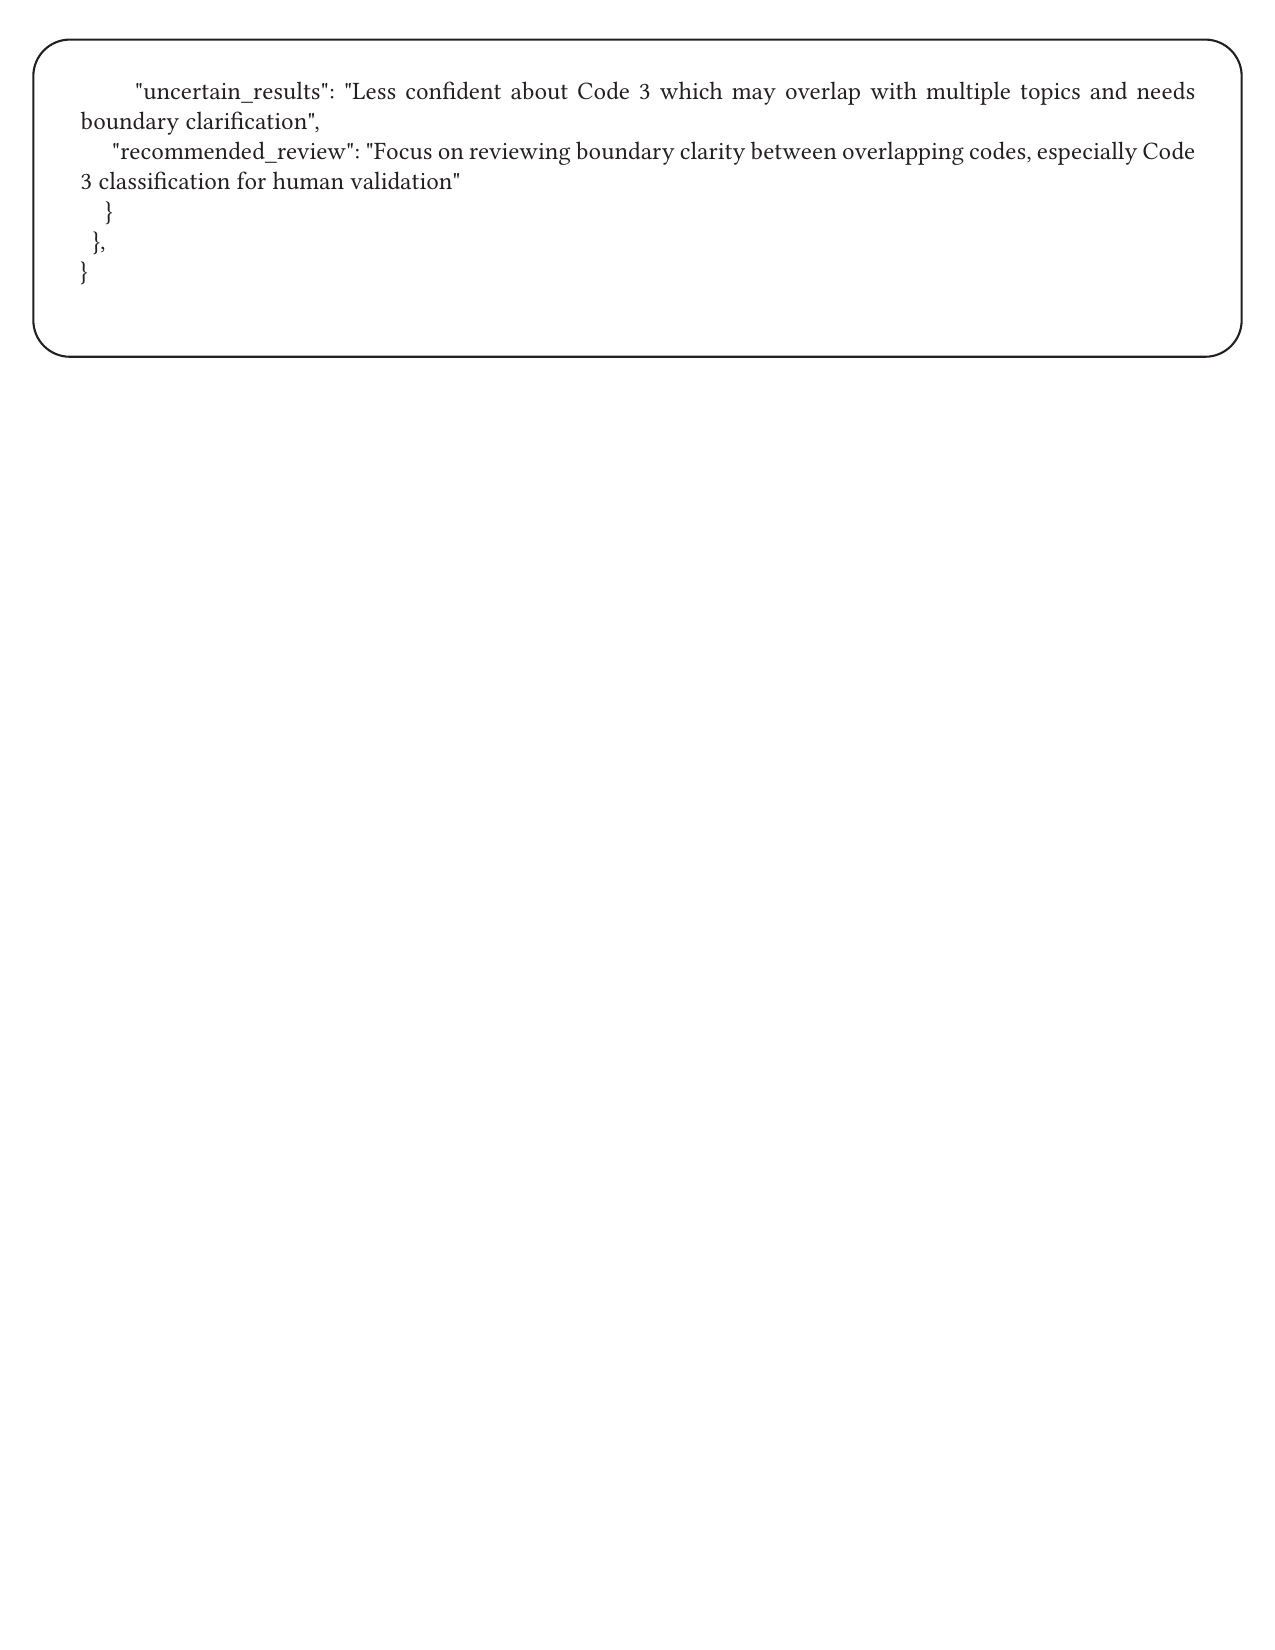}
    % \caption{}
    \label{fig: topic_prompt}
\end{figure*}

\begin{figure*}[!htbp]
    \centering
    \includegraphics[width=\linewidth]{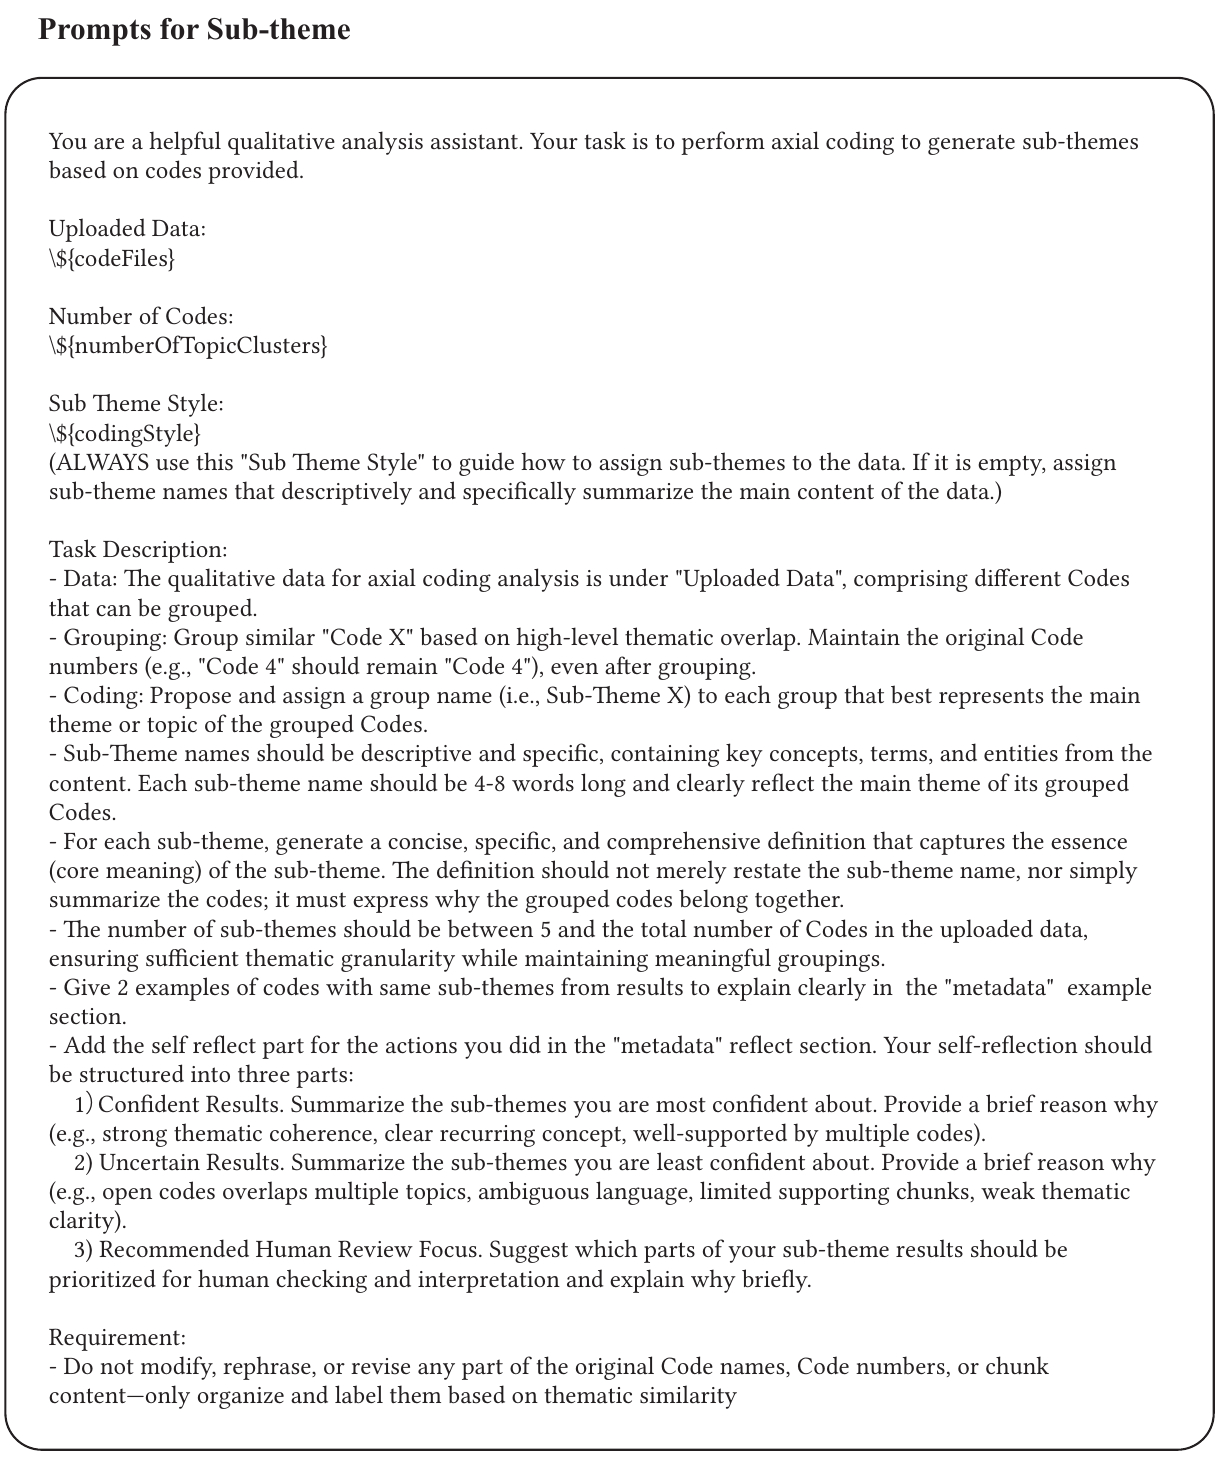}
    % \caption{}
    \label{fig: code_prompt}
\end{figure*}
\begin{figure*}[!htbp]
    \centering
    \includegraphics[width=\linewidth]{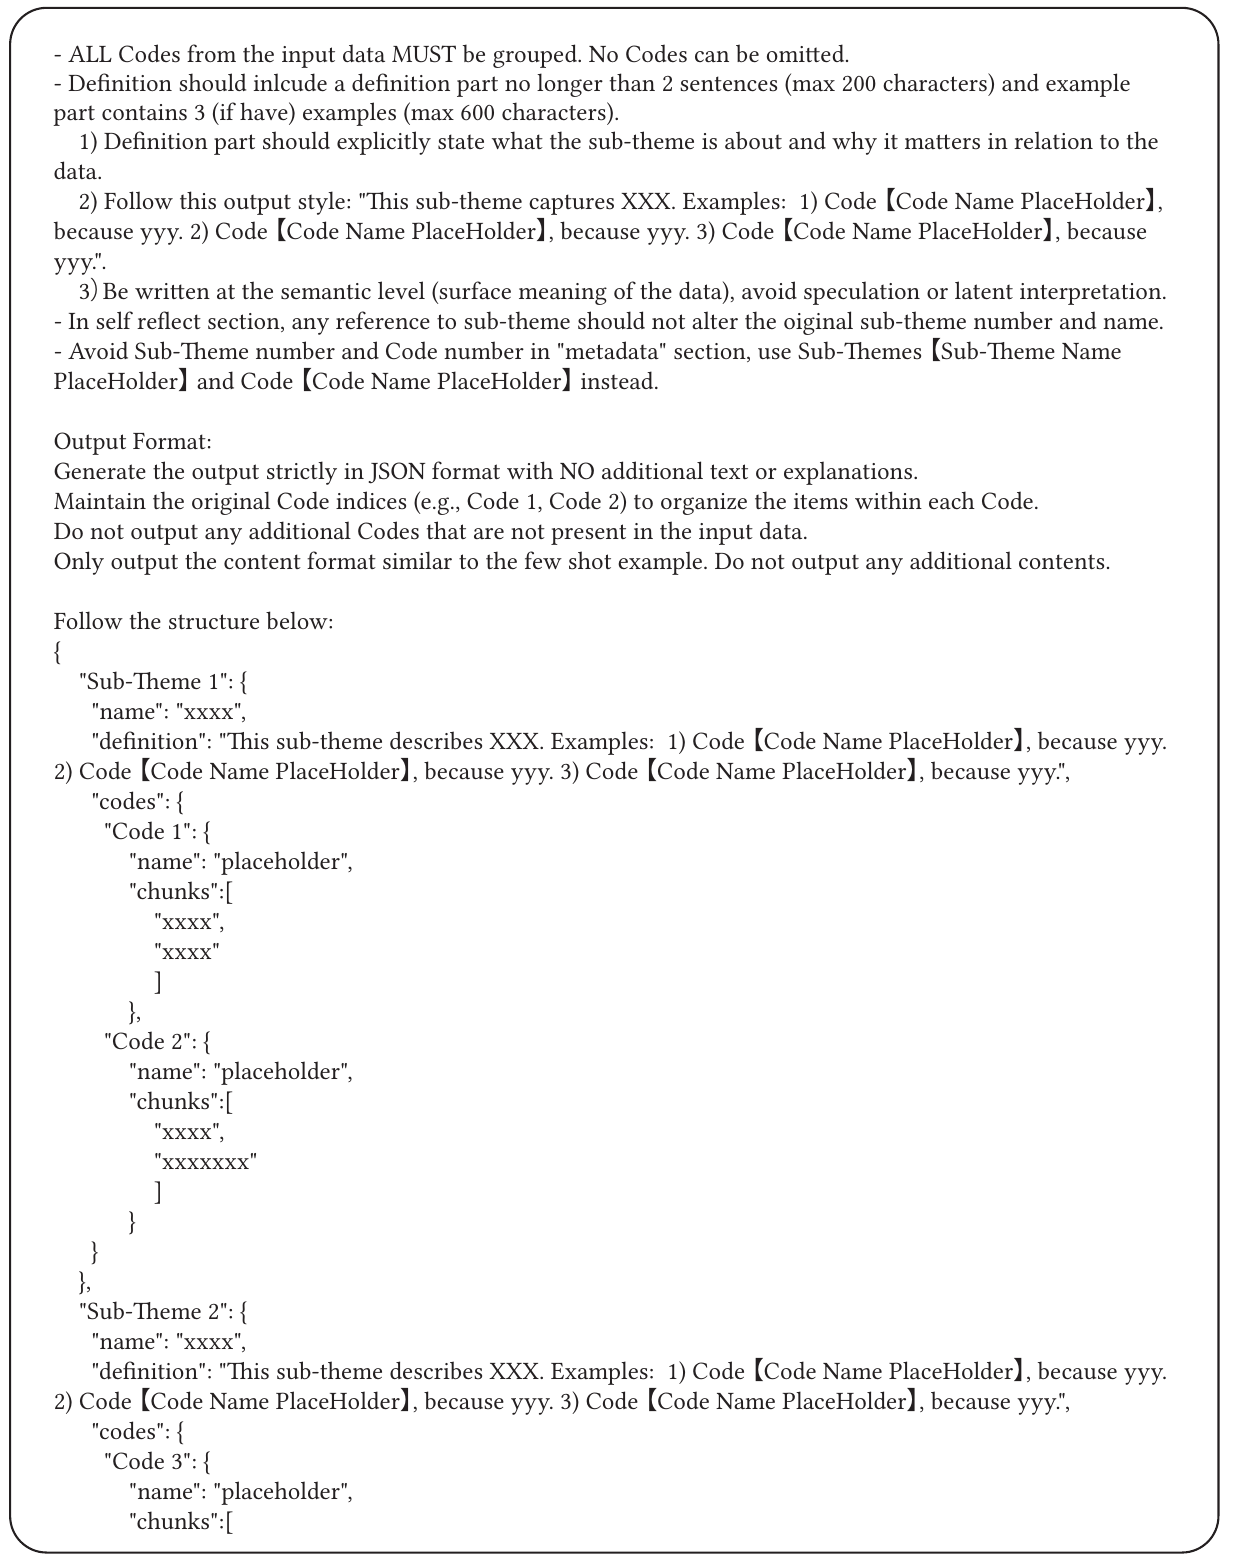}
    % \caption{}
    \label{fig: code_prompt}
\end{figure*}
\begin{figure*}[!htbp]
    \centering
    \includegraphics[width=\linewidth]{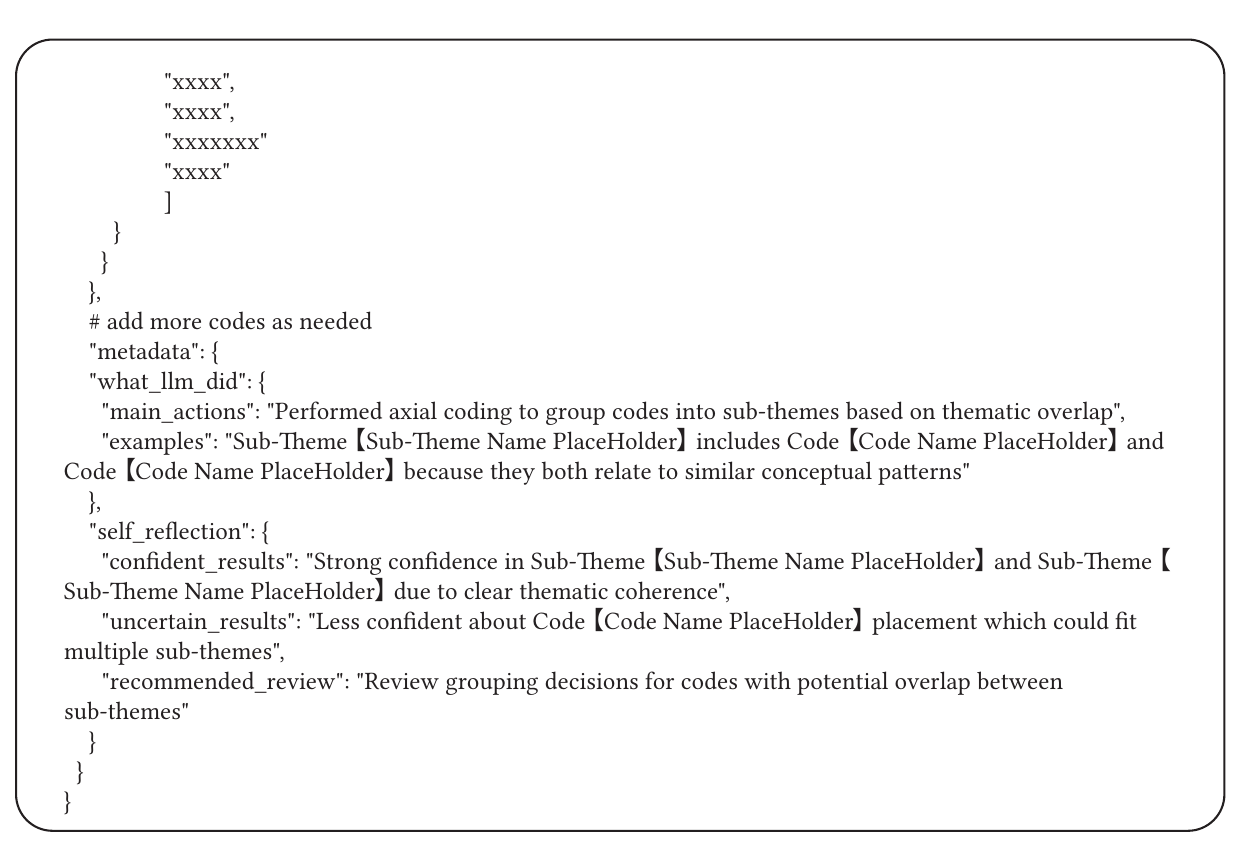}
    % \caption{}
    \label{fig: code_prompt}
\end{figure*}
\begin{figure*}
    \centering
    \includegraphics[width=\linewidth]{Figure/prompt_list/subtheme_prompt_1.pdf}
    % \caption{}
    \label{fig: code_few_shot_prompt}
\end{figure*}
\begin{figure*}
    \centering
    \includegraphics[width=\linewidth]{Figure/prompt_list/subtheme_prompt_2.pdf}
    % \caption{}
    \label{fig: code_few_shot_prompt}
\end{figure*}
\begin{figure*}
    \centering
    \includegraphics[width=\linewidth]{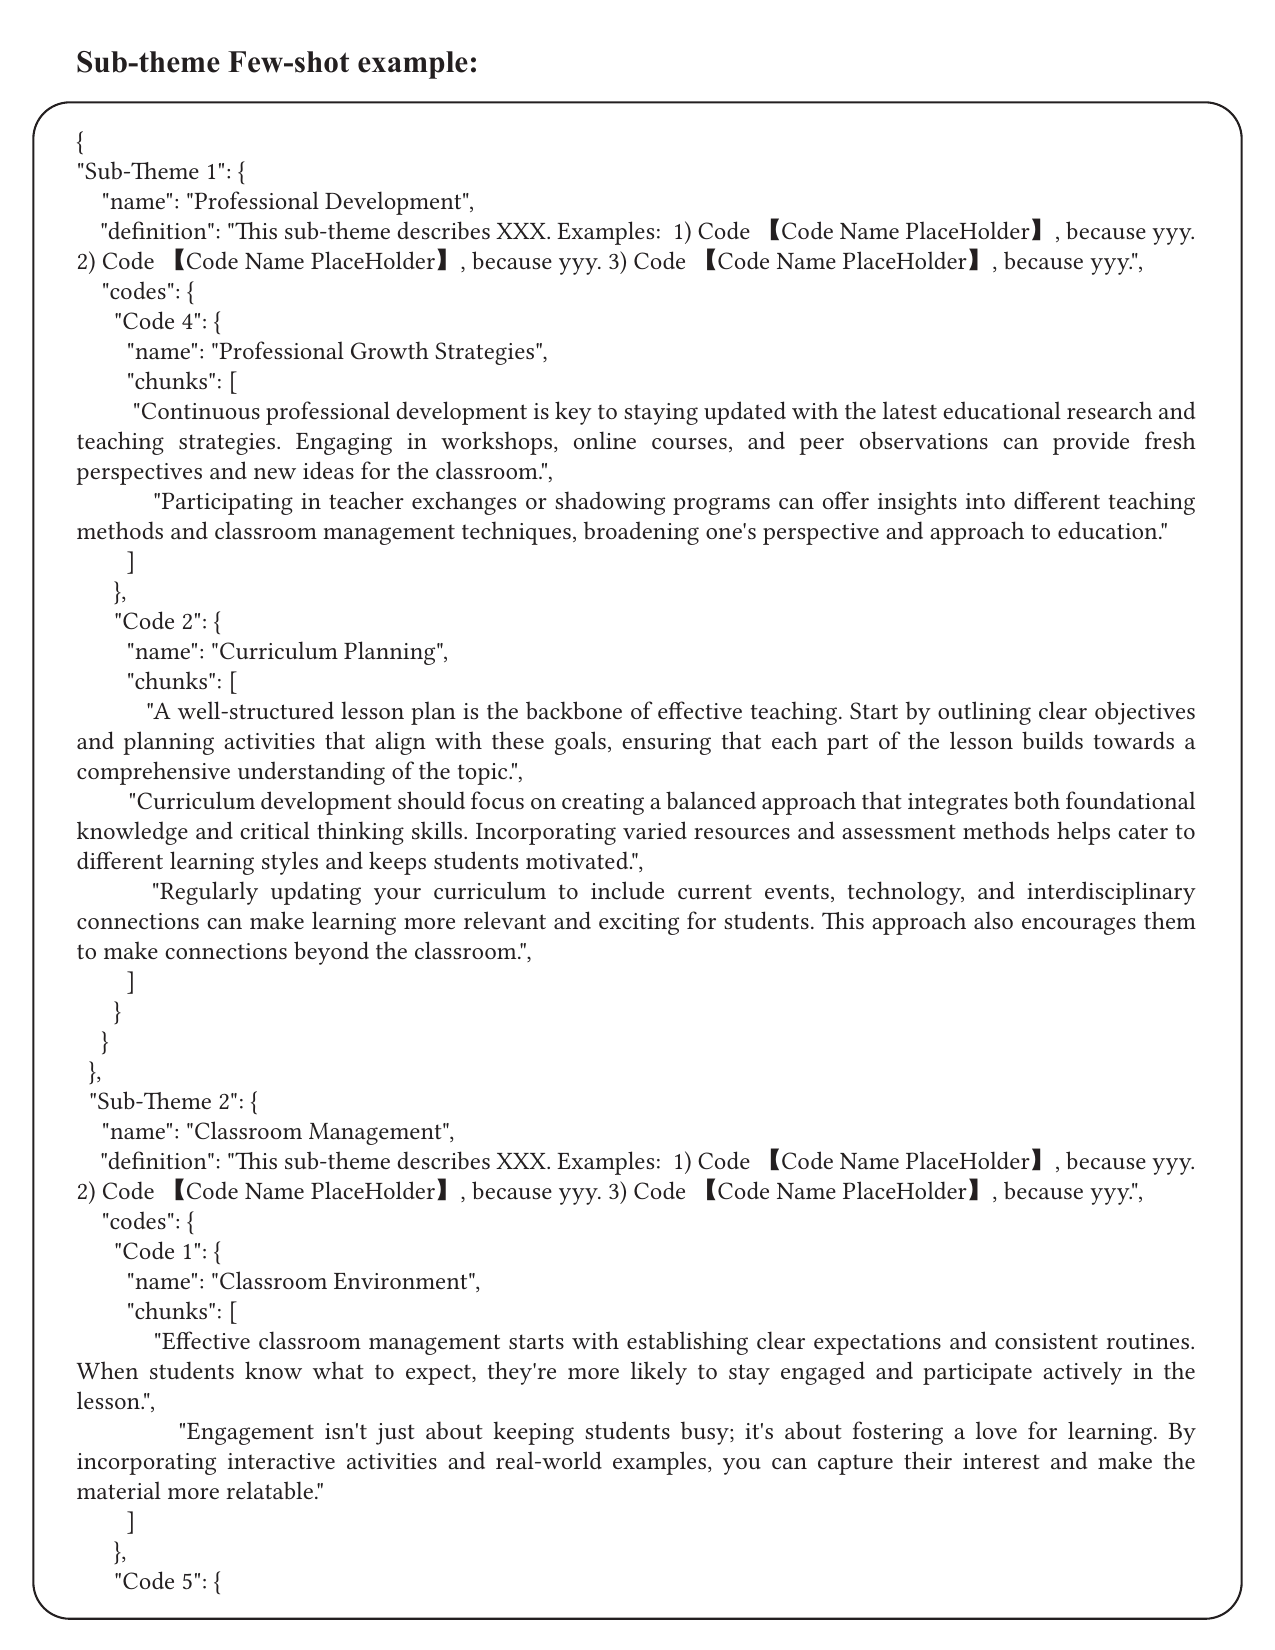}
    % \caption{}
    \label{fig: code_few_shot_prompt}
\end{figure*}
\begin{figure*}
    \centering
    \includegraphics[width=\linewidth]{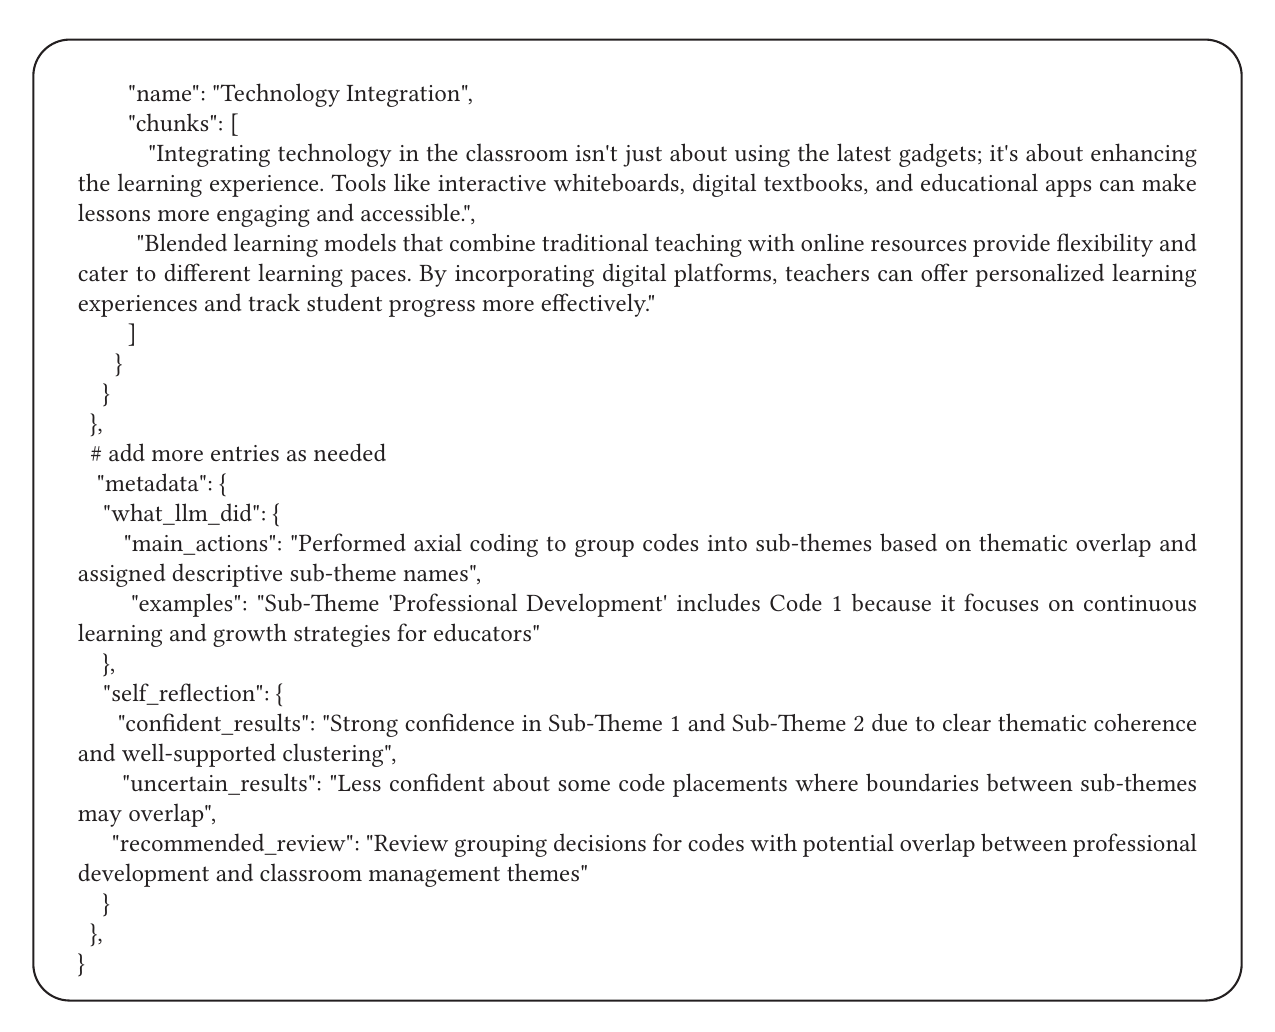}
    % \caption{}
    \label{fig: code_few_shot_prompt}
\end{figure*}

\begin{figure*}[!htbp]
    \centering
    \includegraphics[width=\linewidth]{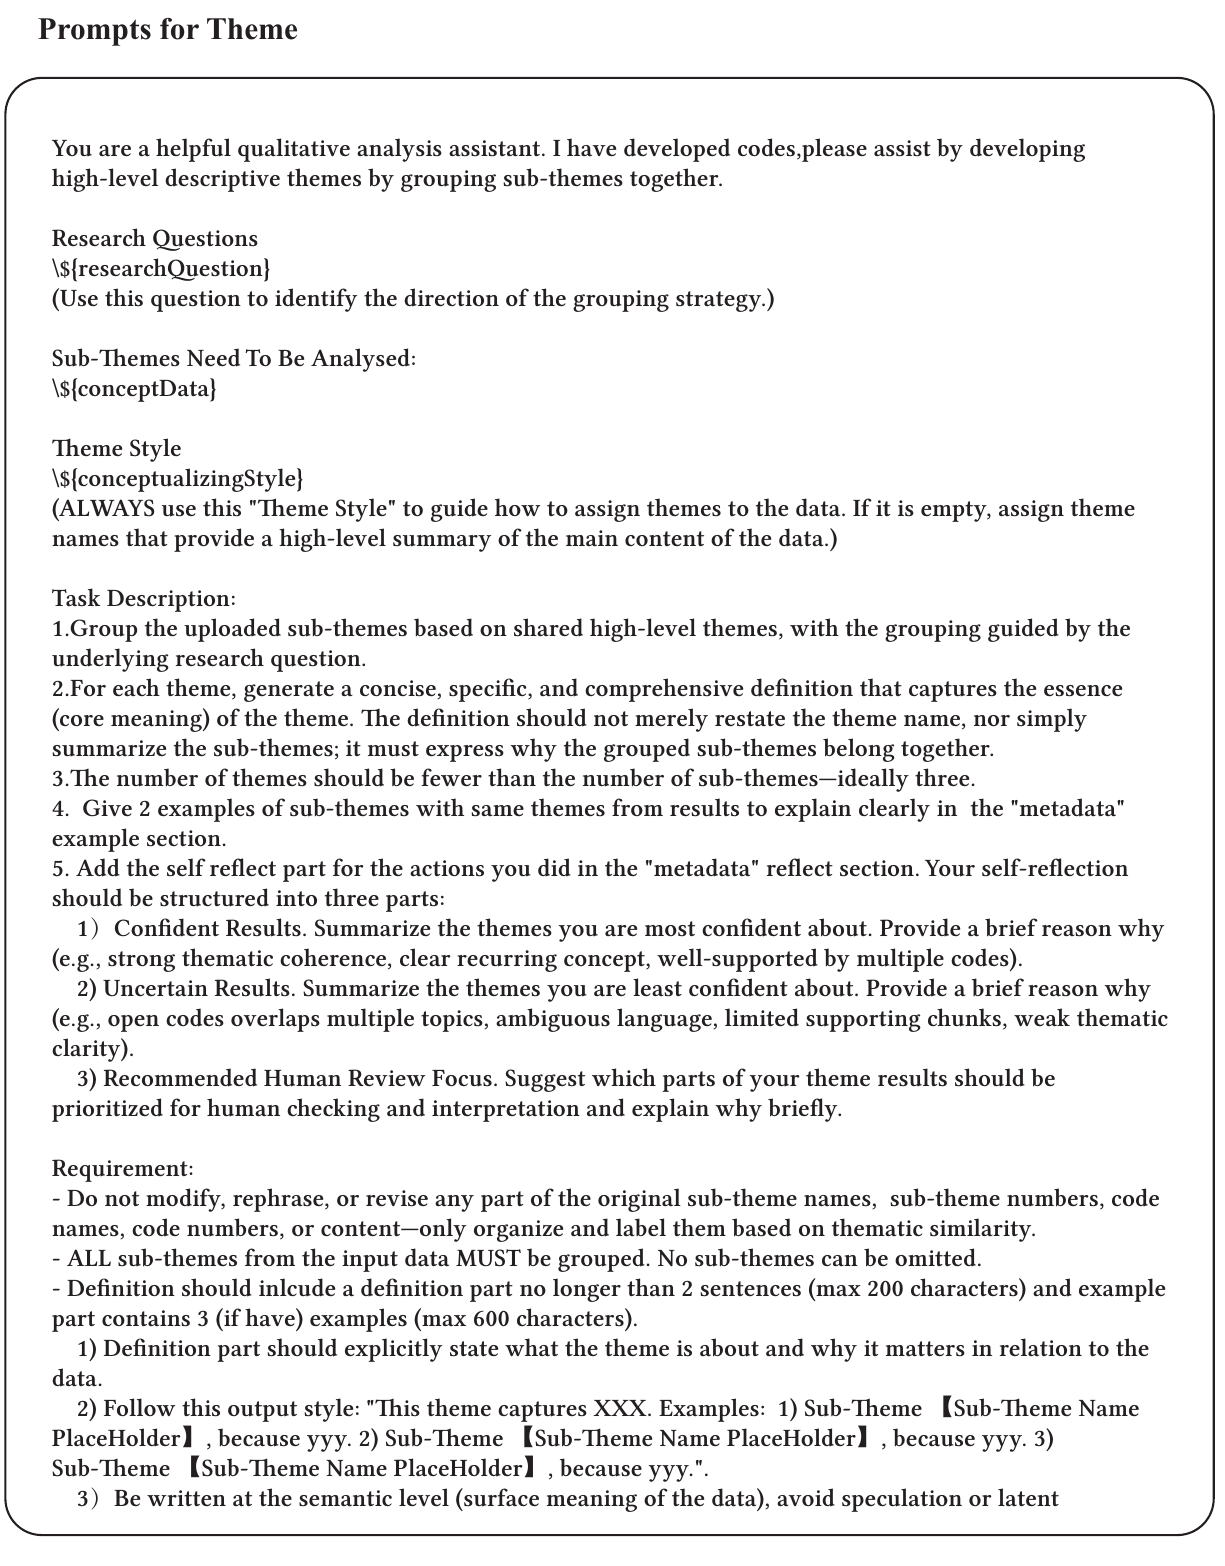}
    % \caption{}
    \label{fig: concept_prompt}
\end{figure*}
\begin{figure*}[!htbp]
    \centering
    \includegraphics[width=\linewidth]{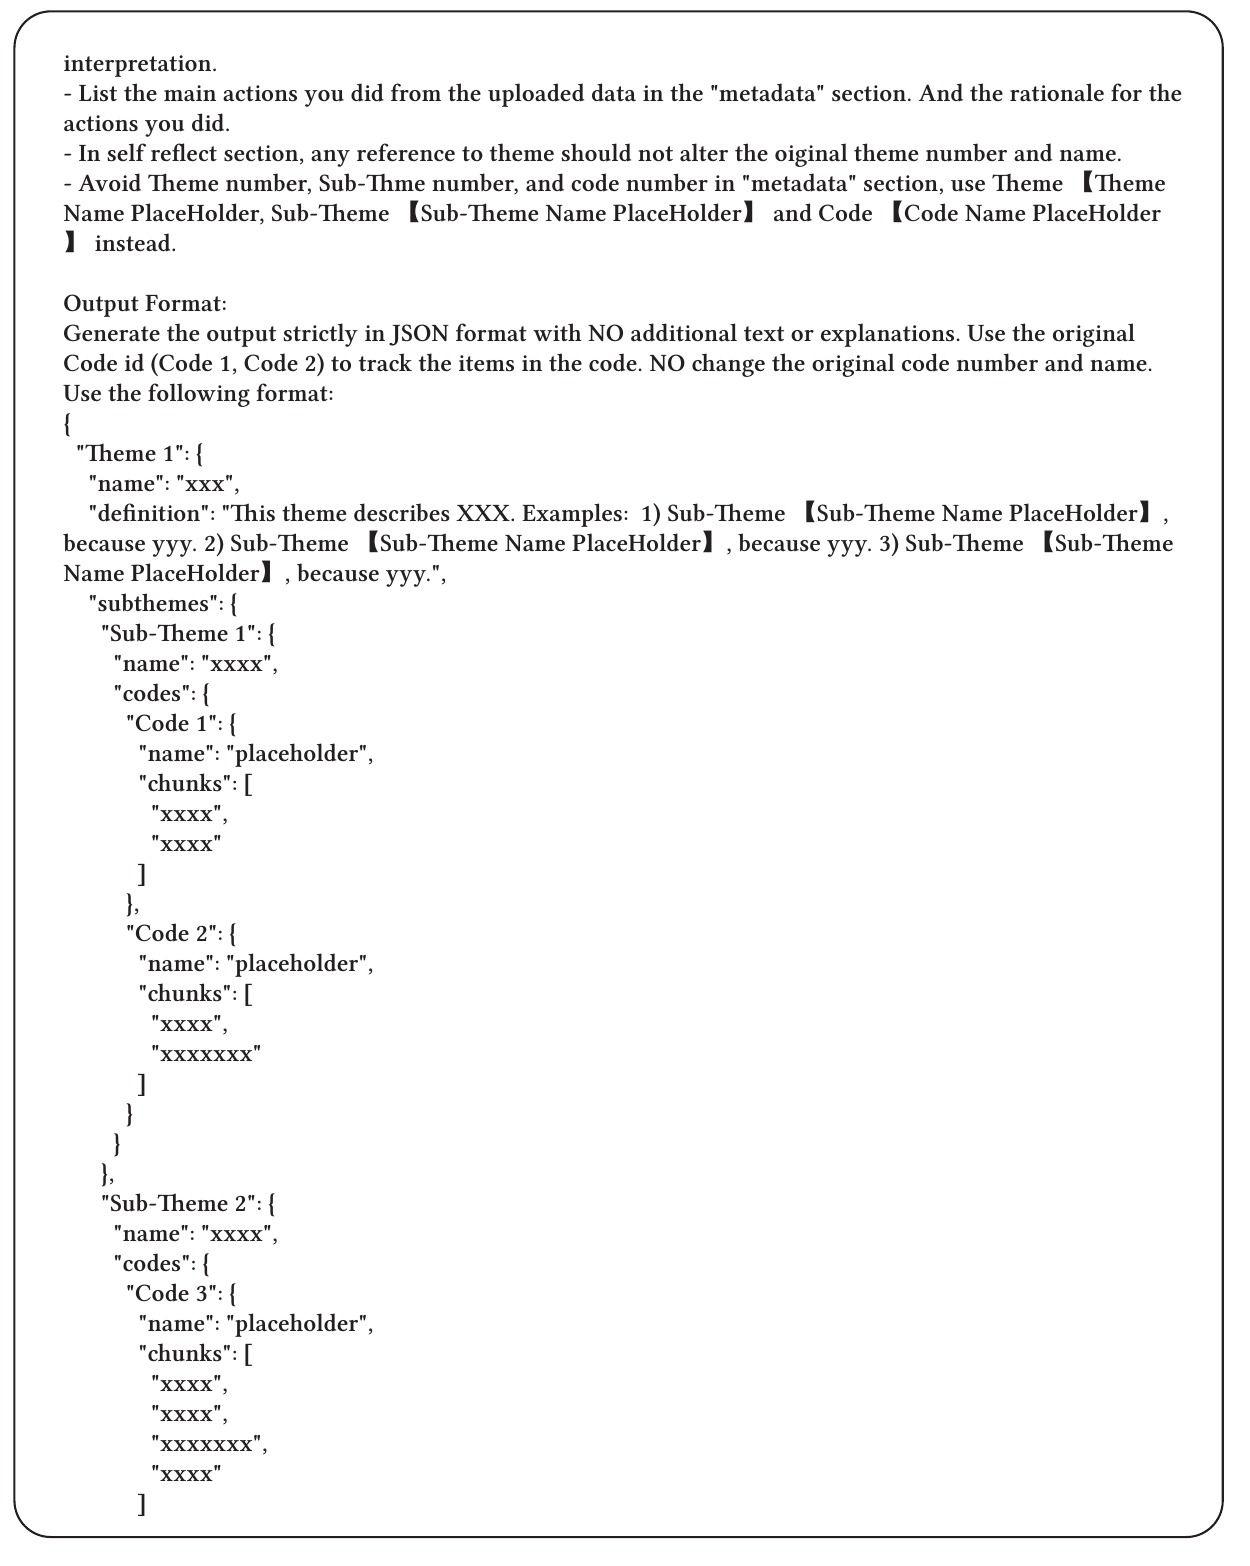}
    % \caption{}
    \label{fig: concept_prompt}
\end{figure*}
\begin{figure*}[!htbp]
    \centering
    \includegraphics[width=\linewidth]{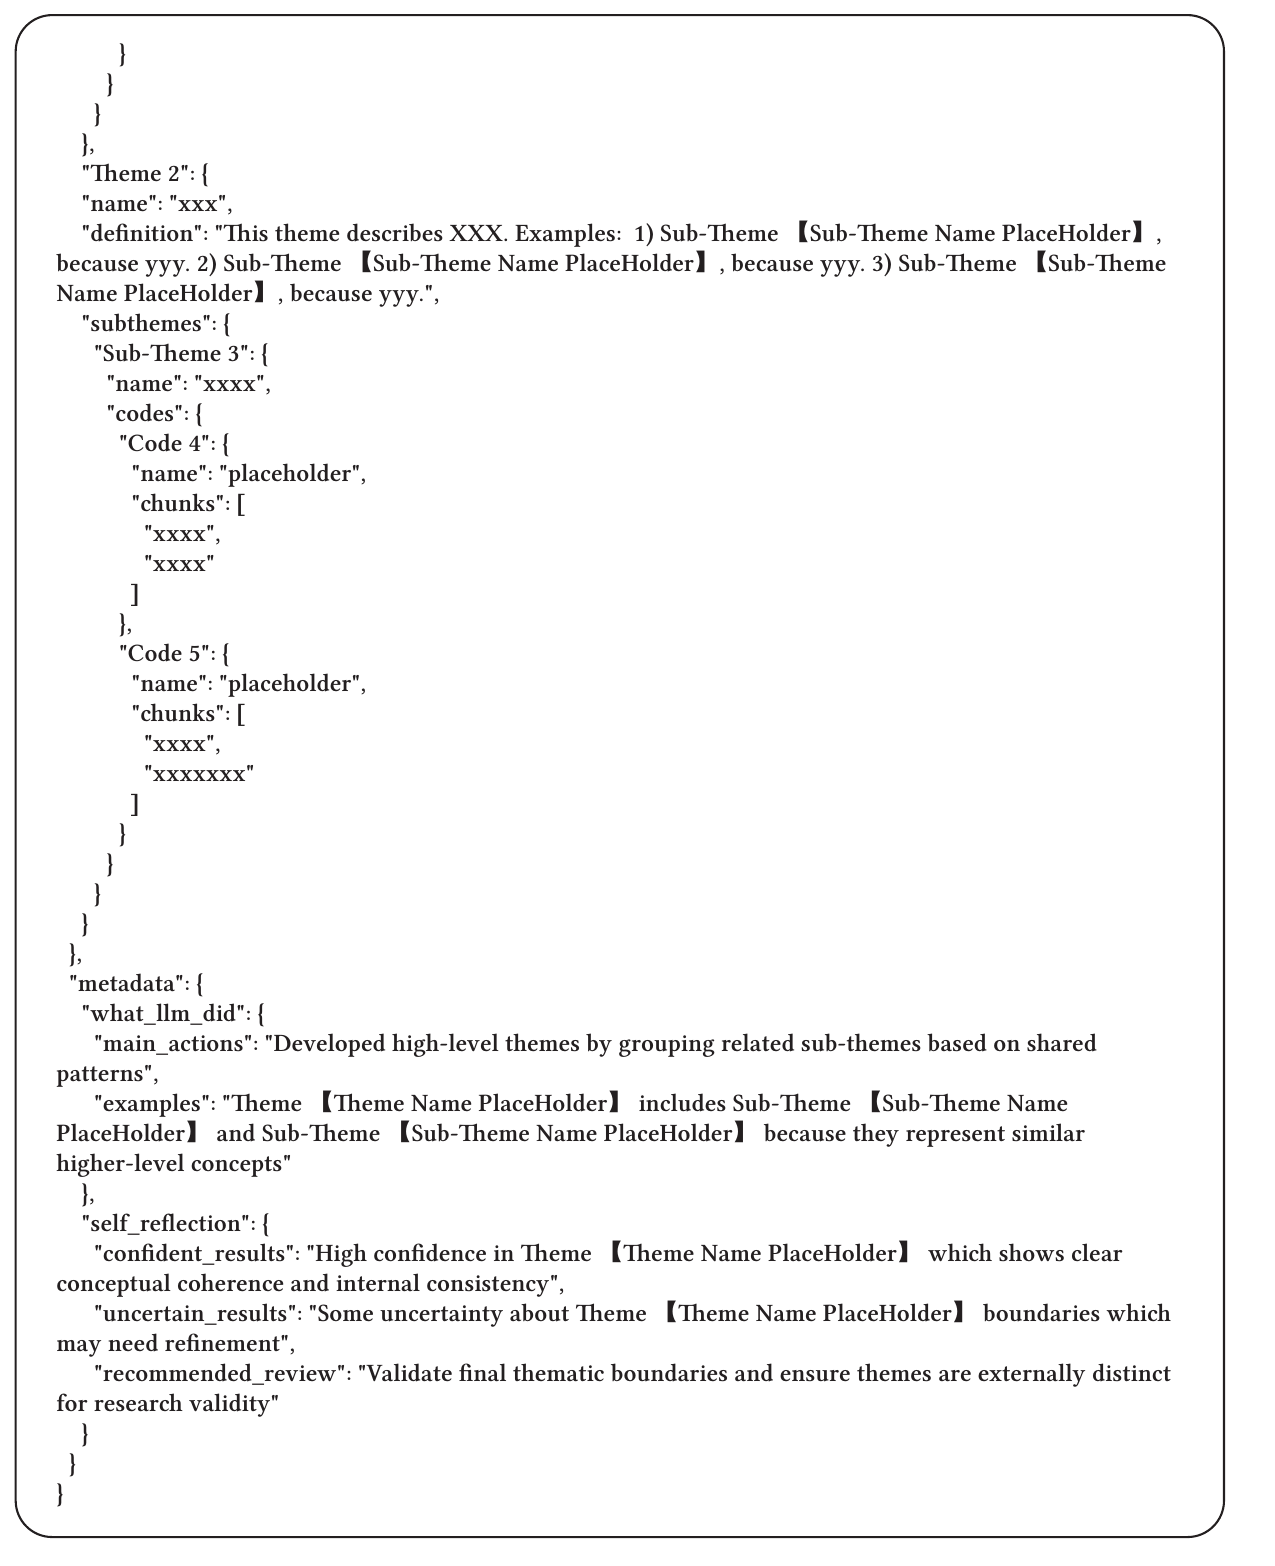}
    % \caption{}
    \label{fig: concept_prompt}
\end{figure*}

\begin{figure*}[!htbp]
    \centering
    \includegraphics[width=\linewidth]{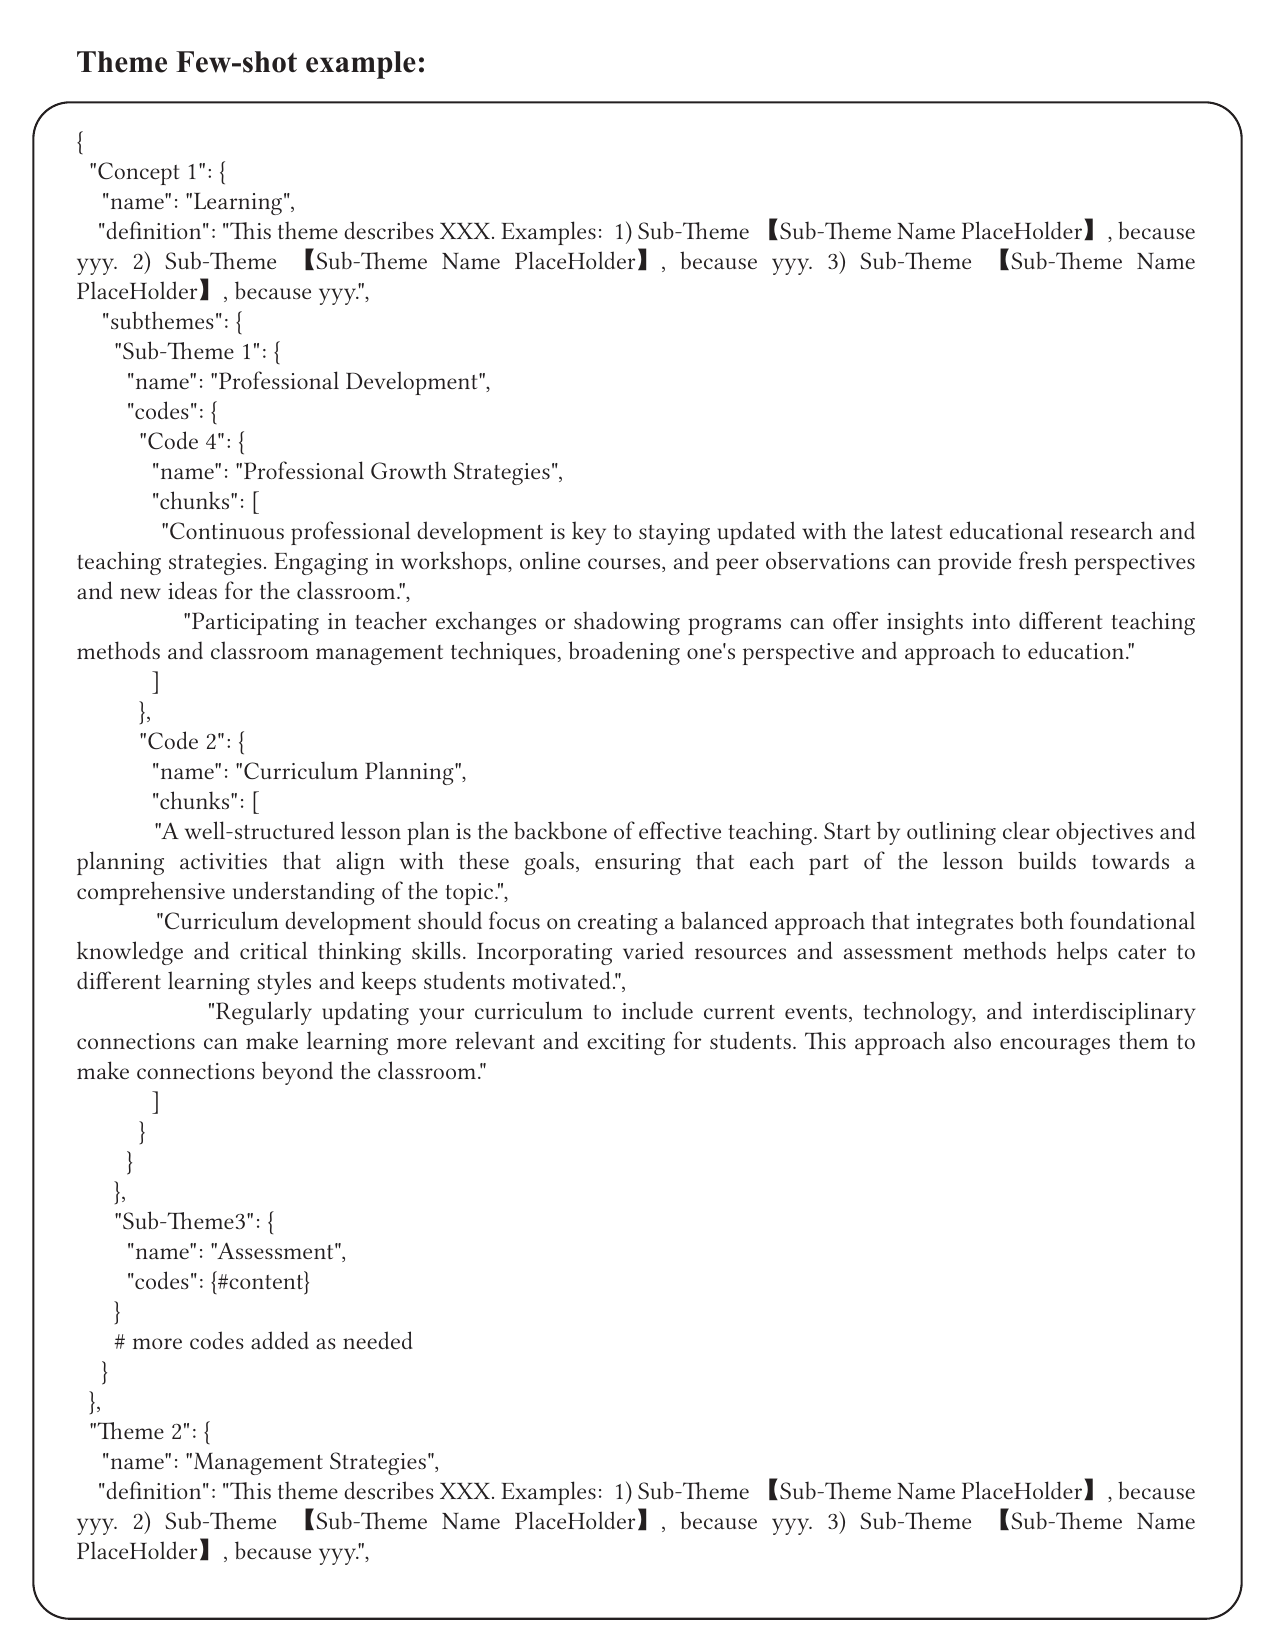}
    % \caption{}
    \label{fig: concept_few_shot_prompt}
\end{figure*}
\begin{figure*}[!htbp]
    \centering
    \includegraphics[width=\linewidth]{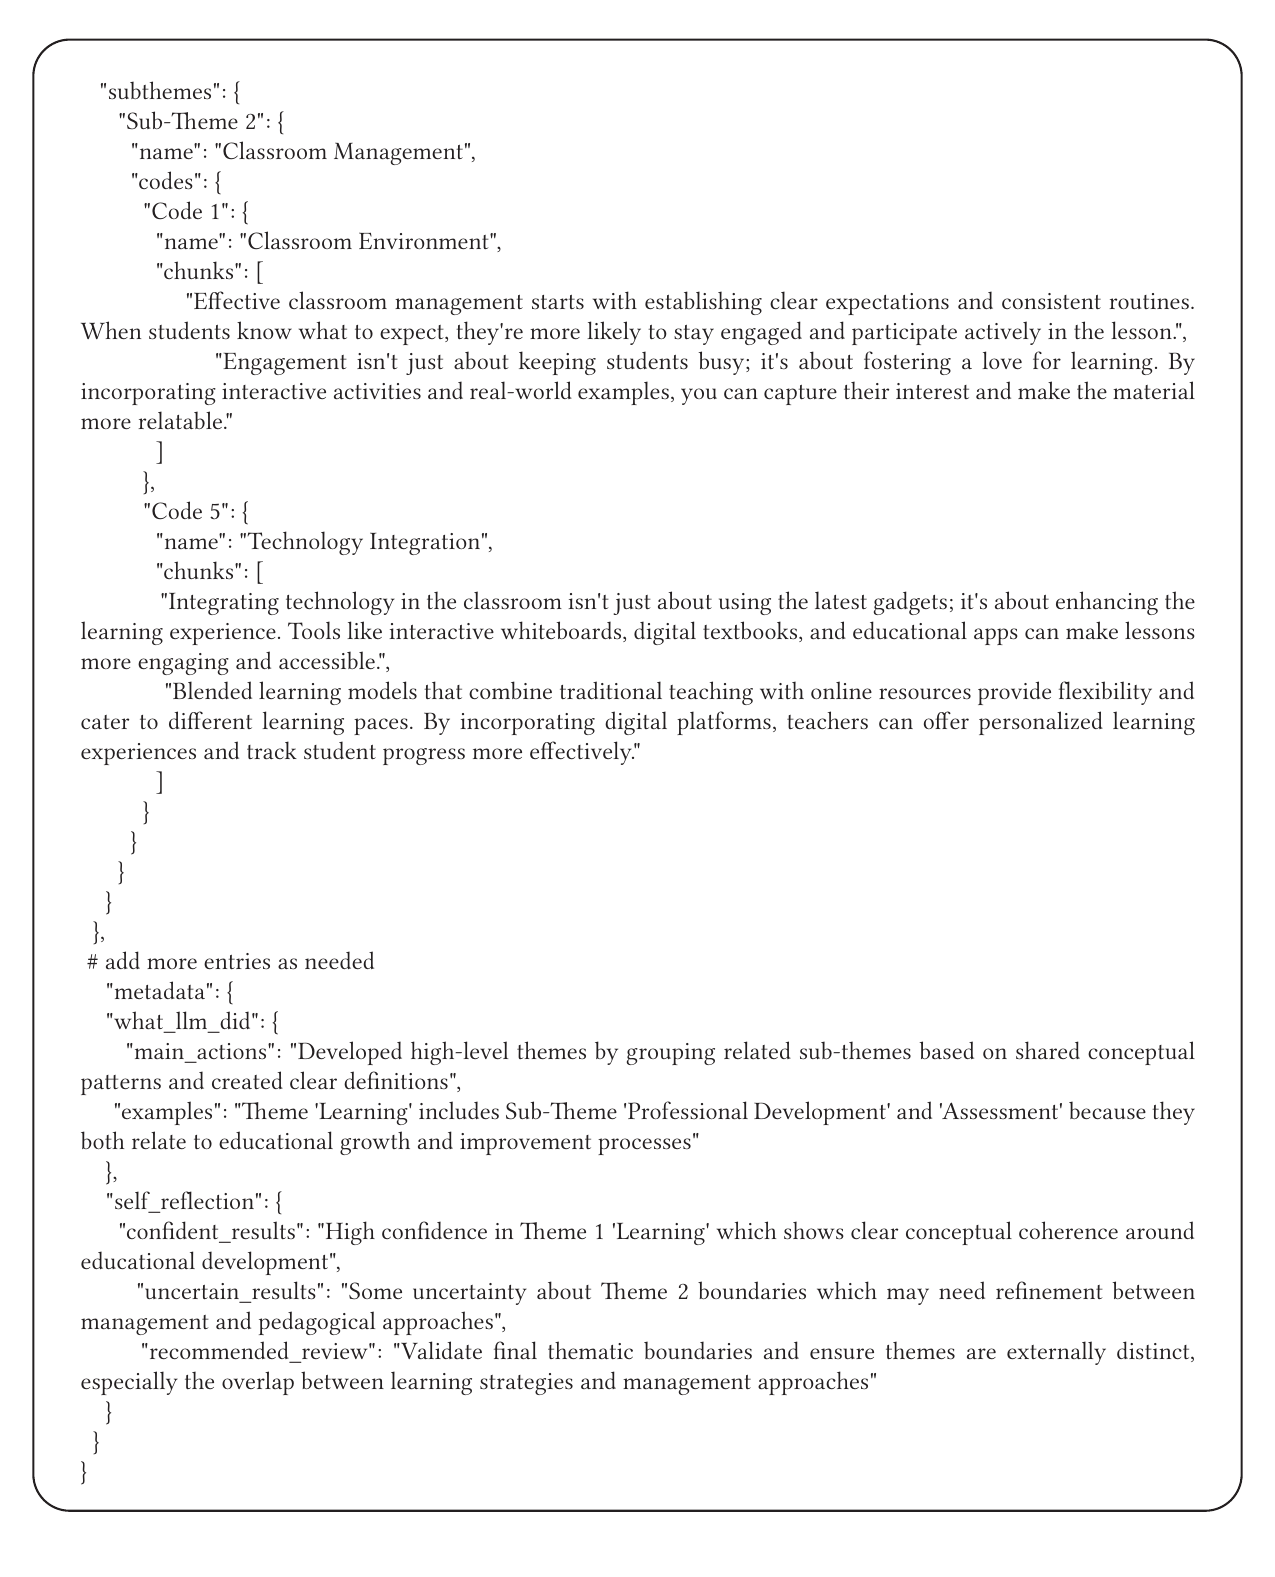}
    % \caption{}
    \label{fig: concept_few_shot_prompt}
\end{figure*}

\begin{figure*}[!htbp]
    \centering
    \includegraphics[width=\linewidth]{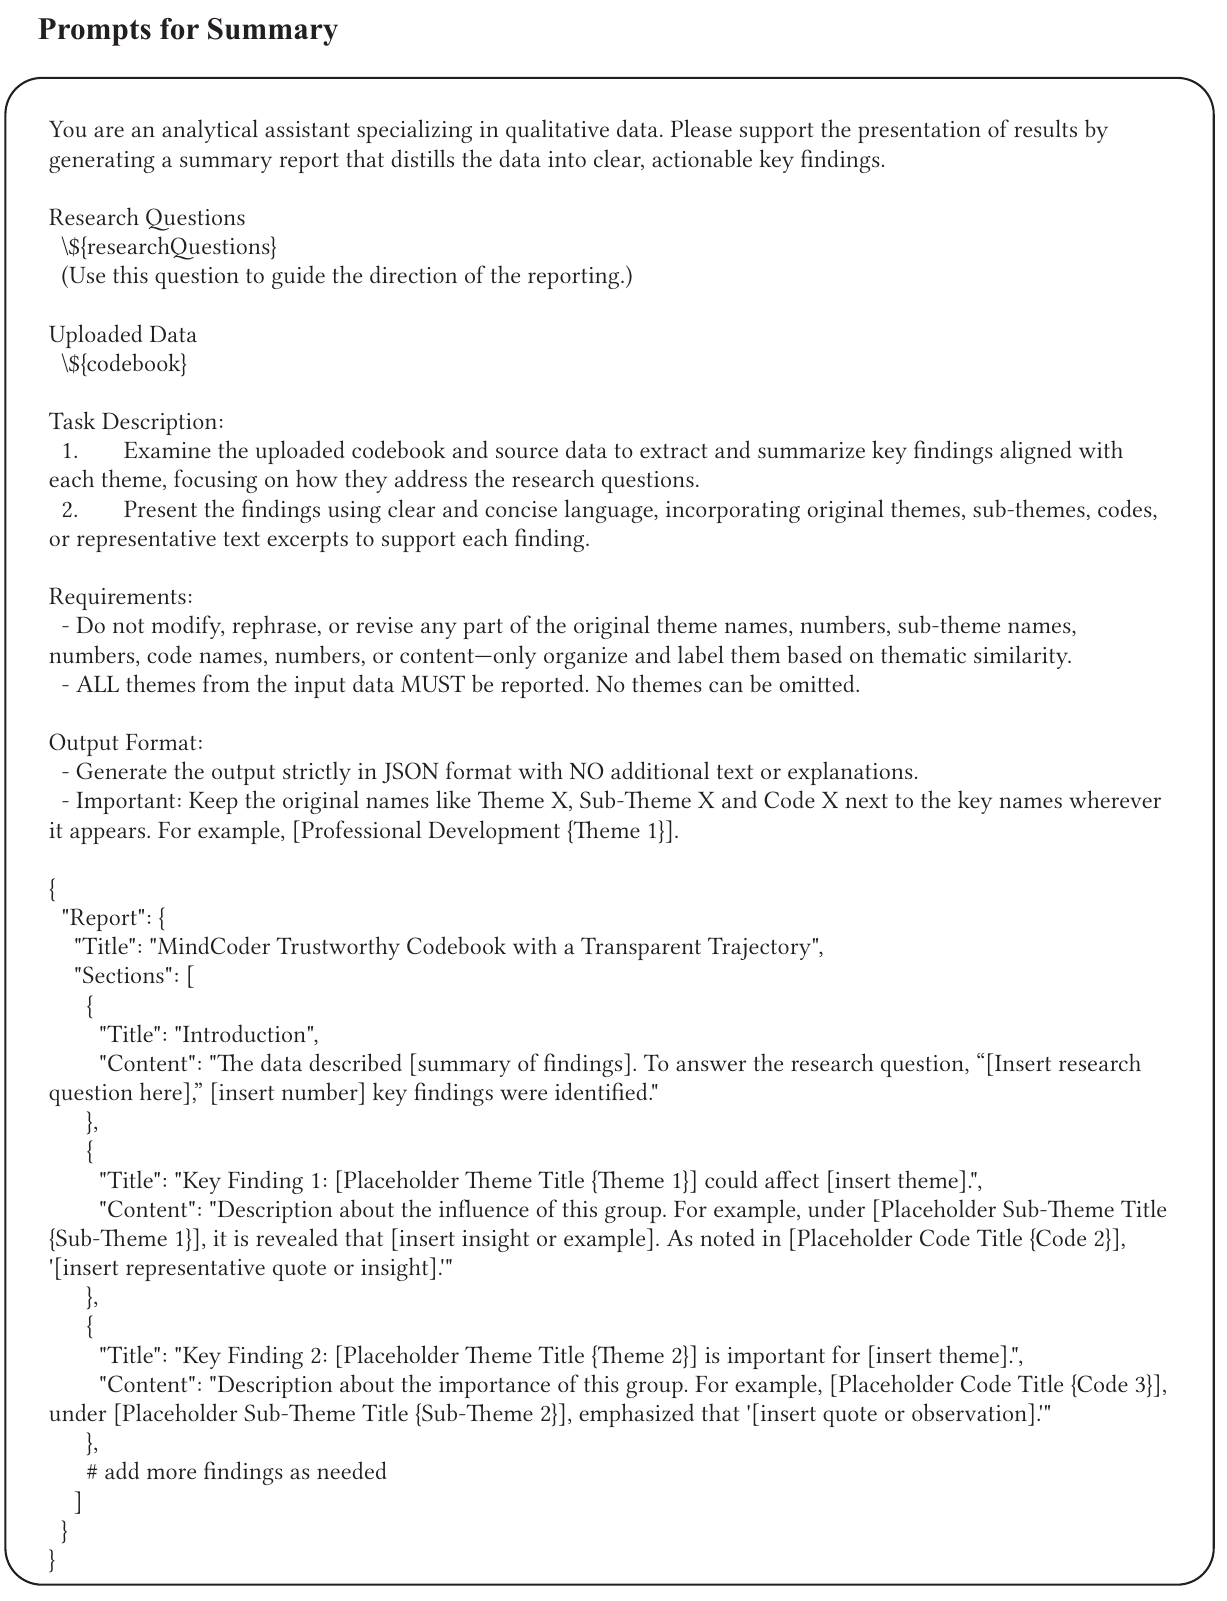}
    % \caption{}
    \label{fig: report_prompt}
\end{figure*}

% \subsection{Prompt for graph annotation}
\begin{figure*}[!htbp]
    \centering
    \includegraphics[width=\linewidth]{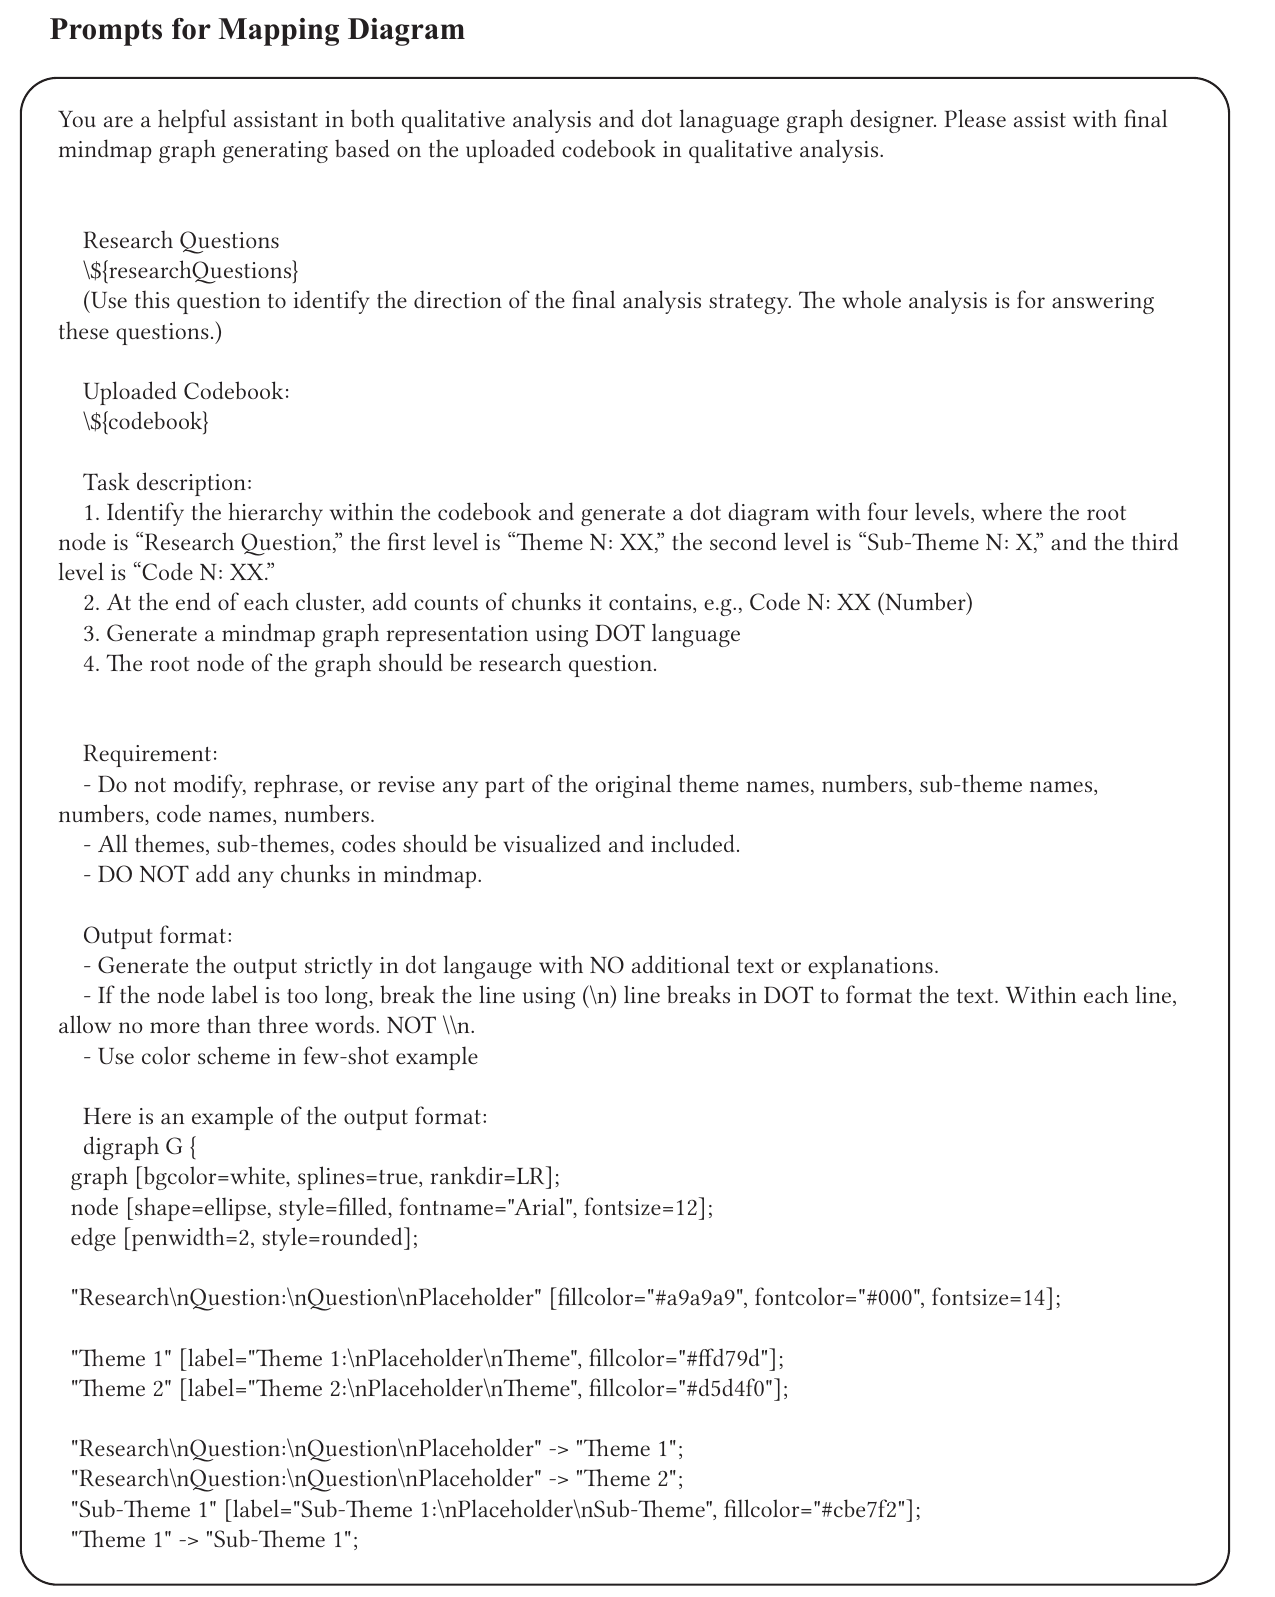}
    % \caption{}
    \label{fig: graph_prompt}
\end{figure*}
\begin{figure*}[!htbp]
    \centering
    \includegraphics[width=\linewidth]{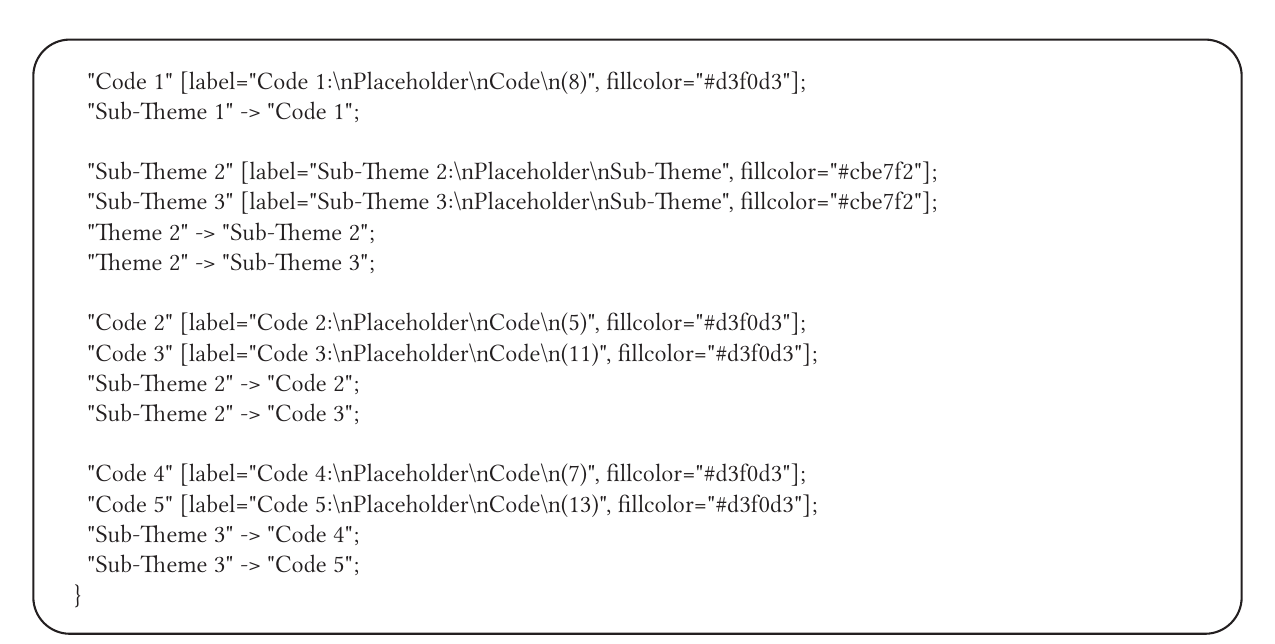}
    % \caption{}
    \label{fig: graph_prompt}
\end{figure*}
